# Supplementary material for: Pre-Trained Multilingual Sequence-to-Sequence Models: A Hope for Low-Resource Language Translation?
Source: arXiv:2203.08850 source file (2022-04-30)
Supplement: Supplementary file 1 [file appendix.tex]

\clearpage
\appendix
\section{Appendix} \label{app:appendix}

\subsection{Corpora used in evaluation}
The JHU Bible Corpus~\cite{mccarthy-etal-2020-johns} is a recently released corpus of Bible translations in over 1600 languages. In several low-resource languages, the Bible is the only available text parallel with another language; moreover, its verse structure makes it multi-parallel across thousands of languages.

The government document corpus~\cite{fernando2020data} is a multilingual corpus for Sinhala--Tamil--English languages on Sri Lankan official government documents, which consists of annual reports, crawled content from government institutional websites, committee reports, procurement documents and acts.

PMIndia~\cite{Barry2020PMIndia} is a parallel corpus of news updates for English and 13 other Indian languages extracted from the Prime Minister of India’s website.

JW300~\cite{agic-vulic-2019-jw300} is a parallel corpus that spans 343 languages obtained from \url{jw.org} including Jehovah Witnesses magazines like Awake and Watchtower. The domain is highly religious but it includes other societal topics, e.g.,  reports about the persecution of their disciples around the world.\footnote{While JW300~\cite{agic-vulic-2019-jw300} has been automatically aligned from  \url{JW.org}, \citet{abbott2019benchmarking} and \citet{alabi-etal-2020-massive} have verified the quality for African languages. For languages with non-Latin scripts in our study, the alignment has been judged to be poor by native speakers.} 

DGT-TM~\cite{tiedemann2012parallel} consists of multilingual translation memory corresponding to the `Summaries of EU legislation'. They are short explanations of the main legal acts passed by the European Union (EU). The type of legislation included in the dataset refers to directives, regulations and decisions, as well as international agreements. The dataset is available in 25 languages.

CCAligned~\cite{el2020massive} and CCMatrix~\cite{schwenk2019ccmatrix} are parallel texts that were automatically aligned using LASER sentence embeddings~\cite{schwenk-2018-filtering}. CCAligned is newer, and has more texts for LRLs. The dataset, although noisy~\cite{qualityAtAGlance}, has been used to develop highly multilingual machine translation models like M2M100~\cite{fan2021beyond} and mBART multilingual MT~\cite{tang2020multilingual}.

\subsection{Model Training Details}

%We used the standard sequence-to-sequence Transformer based architecture \cite{vaswani2017attention} as 
For the mBART50 and mT5-base models, \cite{tang2020multilingual}, %which consists of 12 layers of encoder-decoder with the model dimension of 1024 on 16 heads. For all directions, 
we train up to 3 epochs with \mbox{5\textsc{e}-05} learning rate, 0.1 dropout, 200 as maximum source, target length, and with the batch size of 10. We used beam search with beam size 5 for decoding. The final results are reported in sacreBLEU \cite{post-2018-call}. All the fine-tuning experiments conducted using HuggingFace Transformers\footnote{\url{https://github.com/huggingface/transformers}} library and trained on Tesla V100 machines. 

xWe followed the bilingual fine-tuning on the selected 10 languages pairs. For each pair of language direction we initialize our NMT encoder-decoder with  pre-trained mBART model's corresponding language encoder and decoder. Once we initialized the weights, we continued our training. Instead of random initialization, here our training is started with pre-trained model's weights- this is referred as fine-tuning. By doing this, we try to  fine-tune the pre-trained model parameters for our particular selected translation task.% For the 4 languages that are not supported by mBART50, we applied the related language fine-tuning strategy \cite{madaan2020transfer,cahyawijaya2021indonlg}, where we picked the language that is syntactically close and both are from same language family. We pick Bengali for Assamese, Telugu for Kannada, French for Irish, and Swahili for Yoruba. For the Indian languages Assamese, Kannada, we try to find the best match among other Indian language families, where we found  Assamese are more closely to Bengali and receptivity for Kannada we found Telugu.

Considering the computational memory bottlenecks, we used the mT5-base model, which supports over 100 languages including five out of the six languages we evaluated on. Irish was not supported, therefore, we make use of the French language code for fine-tuning the model.

Transformer model~\cite{vaswani2017attention} was trained using the same datasets used for fine-tuning mBART. We use two transformer architectures. When the data set size is less than 10k the model consists of 3 encoder and decoder layers with embedding dimension of 512 and 2 attention heads. When the data set size is greater than or equal to 10k the model trained consisted of 6 encoder and decoder layers with a embedding dimension of 256 and 2 attention heads. We train the models with SentencePiece sub-wording techniques from scratch. Both the models had an initial learning rate of 1e-03 with a weight decay of 1e-04, dropout of 0.4 and batch size 32.  We trained the model until the validation loss saturated. The model with the lowest validation loss was identified as the best model and used for testing. We used beam search of 5 for decoding. For the training, we use FairSeq\footnote{\url{https://github.com/pytorch/fairseq}} tool. %All the results are reported in sacreBLEU~\cite{post-2018-call}.
 %   We train Transformer model proposed by \cite{} with SentencePiece sub-wording techniques from scratch. We trained the model until the validation loss saturated. The model with the lowest validation loss was identified as the best model and used for testing. For the trainig, we use FairSeq\footnote{\url{https://github.com/pytorch/fairseq}} tool.
    
  %  \item mT5: \citet{liu2021continual}  have shown that mBART has a better overall performance over mT5. In order to further validate that, we ran an initial set of experiments with mT5 as well. We followed the same parameter values as mBART fine-tuning in the Section \ref{}. \st{David, pelase add the details of mt5 fine-tuning}
    
% \flushcolsend
